# Supplementary material for: Hindsight Bias in Clinical Temporal Reasoning: How Future Data Exposure Affects Large Language Model Judgment
Source: arXiv:2609.13454 source file (2026-09-11)
Supplement: Supplementary file 1 [file appendix_roadmap.tex]

\section{Data Collection and Cohort Construction}
\label{app:data}

\paragraph{What to include.}
Document the exact PubMed Central Open Access retrieval date, search queries, publication window, inclusion and exclusion criteria, duplicate handling, language restrictions, and article-license checks. Provide a case-level manifest containing PMC identifier, cohort, publication year, source license, availability of original narrative, human TTS, LLM TTS, questions, and all answer conditions.

\paragraph{Recommended appendix items.}
\begin{itemize}
    \item \textbf{Figure A1:} cohort flow diagram from retrieved reports to the final 40 sepsis and 130 GLP-1/diabetes cases.
    \item \textbf{Table A1:} inclusion/exclusion counts and reasons by cohort.
    \item \textbf{Table A2:} case-level manifest or a link to the machine-readable manifest.
    \item \textbf{Table A3:} publication-year, article-length, and license distributions.
\end{itemize}

\section{TTS Construction, Annotation, and Alignment}
\label{app:tts}

Describe the human annotation protocol, annotator qualifications, training, adjudication, time normalization, handling of uncertain dates, and quality control. Provide the complete LLM-TTS generation prompt, model version, inference settings, repair logic, and validation checks. Define event time, information-availability time, and documentation time, and state which field controls masking.

\begin{itemize}
    \item \textbf{Table A4:} number of events, trajectory duration, event density, and retained fraction at the cutoff for human and LLM TTS by cohort.
    \item \textbf{Table A5:} exact and semantic cutoff-alignment rates between human and LLM TTS.
    \item \textbf{Figure A2:} distributions of TTS length and trajectory duration.
    \item \textbf{Figure A3:} examples of aligned and misaligned human/LLM events.
    \item \textbf{Table A6:} source-order inversions and chronological-order statistics.
\end{itemize}

\section{Question Generation and Quality Control}
\label{app:questions}

Include the complete generation prompt, JSON schema, repair prompt, and all hidden metadata fields. Explain the three evaluation targets, response formats, reasoning categories, reference answer, hindsight trap, and cutoff selection. List every automated and clinical QC criterion.

\begin{itemize}
    \item \textbf{Table A7:} final question counts by cohort, target, format, options type, and reasoning category.
    \item \textbf{Table A8:} exclusion counts for malformed options, invalid traps, ambiguous anchors, leakage, unsupported answers, duplicates, and cutoff failures.
    \item \textbf{Table A9:} clinical-review agreement, adjudication counts, and retained-item rate.
    \item \textbf{Figure A4:} RelPos distribution by cohort and question target.
    \item \textbf{Examples A1--A8:} representative questions covering each format and target category.
\end{itemize}

\section{Prompts, Models, and Reproducibility}
\label{app:prompts}

Provide the complete prompts for question generation, answer generation in every condition, synthetic-narrative generation, free-response judging, paired judging, and all ablations. Record exact model identifiers, checkpoints, providers, serving frameworks, inference dates, temperatures, seeds, context windows, output limits, quantization, hardware, retry policy, and failure counts.

\begin{itemize}
    \item \textbf{Table A10:} model and run configuration.
    \item \textbf{Table A11:} number of requests, retries, failures, tokens, compute, and estimated cost.
    \item \textbf{Table A12:} prompt and code commit hashes for every reported run.
    \item \textbf{Listing A1:} response canonicalization and schema-validation rules.
\end{itemize}

\section{Complete Results Across All Conditions}
\label{app:all_results}

\begin{table*}[t]
\centering
\caption{All condition-level results by model and cohort. Report masked and full Acc and HTR, $\Delta$Acc, $\Delta$HTR, AIR, HBR$_{\mathrm{joint}}$, HBR$_{\mathrm{cond}}$, masked-correct denominator, and 95\% case-clustered bootstrap confidence intervals.}
\label{tab:appendix_all_conditions}
\textcolor{blue}{TBD: Populate after the final rerun.}
\end{table*}

Recommended full-result tables:
\begin{itemize}
    \item \textbf{Table A13:} condition 0 and conditions 1.1--3.2 for every model in sepsis.
    \item \textbf{Table A14:} condition 0 and conditions 1.1--3.2 for every model in GLP-1/diabetes.
    \item \textbf{Table A15:} equal-weight combined-cohort estimates.
    \item \textbf{Table A16:} case-macro versus question-micro aggregation.
    \item \textbf{Figure A5:} forest plot of $\Delta$HTR for all conditions.
    \item \textbf{Figure A6:} per-case distributions of $\Delta$HTR and $\Delta$Acc.
\end{itemize}

\section{Subgroup Analyses}
\label{app:subgroups}

Report all primary metrics stratified by:
\begin{itemize}
    \item response format: free response, categorical multiple choice, ordinal multiple choice, and true/false;
    \item evaluation target: \texttt{accuracy}, \texttt{hindsight\_bias}, and \texttt{both};
    \item reasoning category;
    \item RelPos tertile or prespecified bins;
    \item number and fraction of visible events;
    \item trajectory duration and event density;
    \item cohort, model, and TTS source.
\end{itemize}

Recommended items are Tables A17--A21 and a faceted forest plot. Keep subgroup claims exploratory unless the comparison was prespecified and sufficiently powered.

\section{Answer-Transition Analysis}
\label{app:transitions}

Provide complete transition matrices for each primary model/cohort/TTS combination. Separate correct-to-correct, correct-to-trap, correct-to-other-error, trap-to-correct, other-error-to-correct, and unchanged-other transitions.

\begin{itemize}
    \item \textbf{Table A22:} transition counts and percentages with denominators.
    \item \textbf{Figure A7:} transition heatmaps by model and cohort.
    \item \textbf{Figure A8:} stacked transition decomposition, emphasizing harmful and beneficial changes.
\end{itemize}

\section{Sensitivity Analyses and Baselines}
\label{app:sensitivity}

Each sensitivity analysis should state its hypothesis, eligible subset, sample size, and effect on the primary conclusions. Include:
\begin{enumerate}
    \item structured-response-only analysis;
    \item clinician-approved-question subset;
    \item exact or high-confidence human--LLM cutoff-aligned subset;
    \item exclusion of prompt-development cases;
    \item question-only baseline;
    \item same-input repeatability and stochastic-instability baseline;
    \item explicit temporal anchor versus unanchored question;
    \item chronological order versus source order and, if used, random order;
    \item context-length placebo;
    \item outcome-only versus non-outcome evidence suffix;
    \item counterfactual-outcome subset;
    \item matched masked/full synthetic narratives;
    \item hard masking versus temporal instruction or boundary marking;
    \item recent-case, paraphrased, and low-identifiability contamination subsets;
    \item alternate HBR definitions and ambiguous free-response scores set to 0, 0.5, and 1.
\end{enumerate}

\begin{itemize}
    \item \textbf{Table A23:} one-row summary of each sensitivity analysis with $\Delta$HTR and conditional HBR.
    \item \textbf{Figure A9:} robustness forest plot comparing all sensitivity estimates with the primary estimate.
\end{itemize}

\section{Free-Response Judge Validation}
\label{app:judge}

Document the judging rubric, blinding, answer-order randomization, model versions, and adjudication procedure. Compare GPT-5.6, a second judge model, and clinicians on a stratified sample.

\begin{itemize}
    \item \textbf{Table A24:} agreement for correctness, trap match, semantic equivalence, and HBR.
    \item \textbf{Table A25:} primary free-response metrics under each judge.
    \item \textbf{Figure A10:} confusion matrices or calibration plots for judge scores against clinician labels.
\end{itemize}

\section{Qualitative Error Analysis}
\label{app:qualitative}

Include a balanced set of examples rather than only failures supporting the hypothesis:
\begin{itemize}
    \item clear correct-to-trap reversals;
    \item correct-to-other-error changes;
    \item beneficial error-to-correct updates;
    \item stable correct answers despite outcome exposure;
    \item suspected prefix leakage;
    \item human/LLM TTS alignment failures;
    \item judge disagreements;
    \item cases suggestive of memorization.
\end{itemize}

For every example, show the reference time, abbreviated prefix, relevant suffix, question, options, reference answer, trap, masked answer, full answer, scores, and a short clinical adjudication.

\section{Contamination, Licensing, Ethics, and Release}
\label{app:ethics}

Report article publication dates, identifying-metadata removal, paraphrase checks, and any retrieval-based contamination analysis. Provide a license manifest and distinguish source text that can be redistributed from derived metadata that can be released independently. Include the IRB approval, exemption, or non-human-subjects determination; data and code availability; model-provider data-use considerations; and anticipated misuse or deployment limitations.

\section{Reproducibility Checklist}
\label{app:reproducibility}

End the appendix with a compact checklist confirming availability of:
\begin{itemize}
    \item case manifest and split definition;
    \item prompts and schemas;
    \item raw and canonicalized responses;
    \item question-level evaluation rows;
    \item bootstrap and plotting scripts;
    \item model and run metadata;
    \item environment or dependency lock file;
    \item code commit and dataset version;
    \item documentation for reproducing every main table and figure.
\end{itemize}
